# Supplementary material for: A Comprehensive Study of Knowledge Editing for Large Language Models
Source: arXiv:2401.01286 source file (2024-11-17)
Supplement: Supplementary file 1 [file appendix.tex]

%%%%%%%%%%%%%%%%%%%%%%%%%%%%%%%%%%%%%%%%%
\hrule height 4pt
\vskip 0.25in
\vskip -\parskip
%%%%%%%%%%%%%%%%%%%%%%%%%%%%%%%%%%%%%%%%%

\vbox{
    \centering
    \LARGE 
    \textbf{Supplementary Materials for \\  
     Knowledge Editing for Large Language Models}
}
%%%%%%%%%%%%%%%%%%%%%%%%%%%%%%%%%%%%%%%%%
\vskip 0.29in
\vskip -\parskip
\hrule height 1pt
% \vskip 0.09in
% \vskip 0.15in
%%%%%%%%%%%%%%%%%%%%%%%%%%%%%%%%%%%%%%%%
 % remove the separator line

\section{Experiment Setting}
We conduct 
\subsection{hparameters for experiment}
